# Supplementary material for: Cubic BeB$_2$: A metastable $p$-type conductive material from first principles
Source: arXiv:2506.00769 source file (2025-09-29)
Supplement: Supplementary file 1 [file BeB2_supplemental.pdf]

# Supplemental information

# Cubic $BeB_2$: A metastable *p*-type conductive material from first principles

Xiao Zhang,[1] Shashi Mishra,[2] Roxana Margine,[2] and Emmanouil Kioupakis[1]

[1] *Department of Materials Science and Engineering, University of Michigan, Ann Arbor, Michigan, 48109, USA*

[2] *Department of Physics, Applied Physics and Astronomy, Binghamton University-SUNY, Binghamton, NY 13902, USA*

(Dated: May 31, 2025)

## I. ELECTRONIC AND PHONON BAND STRUCTURE OF *c*-$BEB_2$ UNDER HIGH PRESSURE

Due to the high-pressure metastable nature of *c*-$BeB_2$, we evaluate its electronic and vibrational properties at 80 GPa. At this elevated pressure, the CBM is notably affected, while the VBM remains largely unchanged. Phonon band structure shows a similar dispersion, with the phonon frequencies increased by a factor of approximately 1.3 at a pressure of 80 GPa. While the ultrahigh pressure is very challenging for experimental perspective, other mechanisms, such as substrate lattice match, are much more promising to overcome the energy barrier of approximately 100 meV/atom.

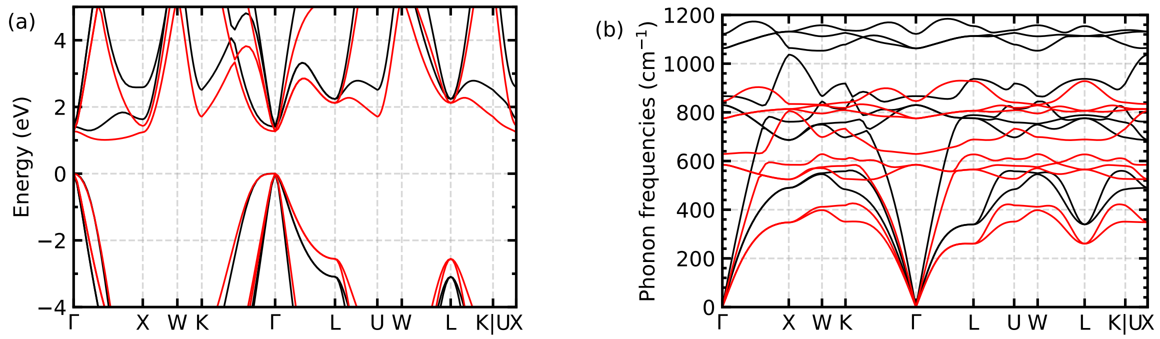


FIG. S1. Electronic and phonon band structure of $c$-$BeB_2$ at ultrahigh pressure of 80 GPa (black) compared to that of zero pressure (red). While the conduction band minimum shows a notable difference, the valence band maximum remains similar. Larger phonon frequencies are observed under high pressure, which is expected due to the more compact structure.

## II. ELECTRONIC BAND STRUCTURE WITH PBE AND HSE EXCHANGE CORRELATION FUNCTIONALS

In this section, we compare the calculated electronic structure of $c$-$BeB_2$ using both the PBE exchange correlational functional and HSE hybrid functional, as shown in Fig. S2. The valence band maximum (VBM) is aligned to zero on the y-axis in both cases to facilitate direct comparison of the electronic band structures. Overall, the inclusion of 25% Hartree-Fock exact exchange in the HSE functional leads to a band widening and a slight change in the effective mass at the VBM, as detailed in Table II of the main text. However, the overall dispersion profile of both the VBM and conduction band minimum (CBM) remain largely unchanged.

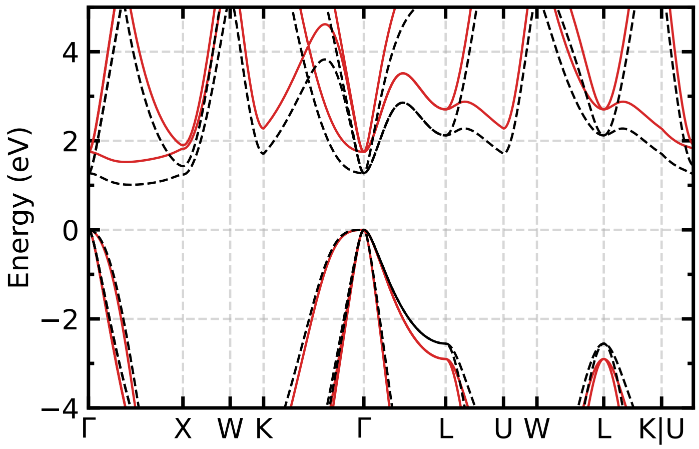


FIG. S2. Calculated electronic band structure of $c$-$BeB_2$ using the PBE (black dashed) and HSE (solid red). HSE results in a widened band gap while inducing only a minor change in the hole effective mass near the VBM.

## III. CALCULATION ABSORPTION COEFFICIENT OF $c$-BEB$_2$

In this section, we show the calculated absorption coefficient of $c$-BeB$_2$ for the intrinsic material and hole concentration of $10^{21}$ cm$^3$ and $10^{22}$ cm$^3$. Figure S3 shows the absorption coefficient evaluated by considering the relationship between the complex refractive index and complex dielectric function: $\tilde{n} = n + i\kappa = \sqrt{\varepsilon_1 + i\varepsilon_2}$, and the absorption coefficient, given by $\alpha(\omega) = \frac{2\omega\kappa}{c}$. We show that the absorption coefficient of the material exceed $2\times10^5$ cm$^{-1}$ above a photon energy of 2 eV regardless of the doping level. Although heavy doping increases the lowest valence to conduction transition onset, the strong sub-gap absorption renders the material not transparent in the visible region.

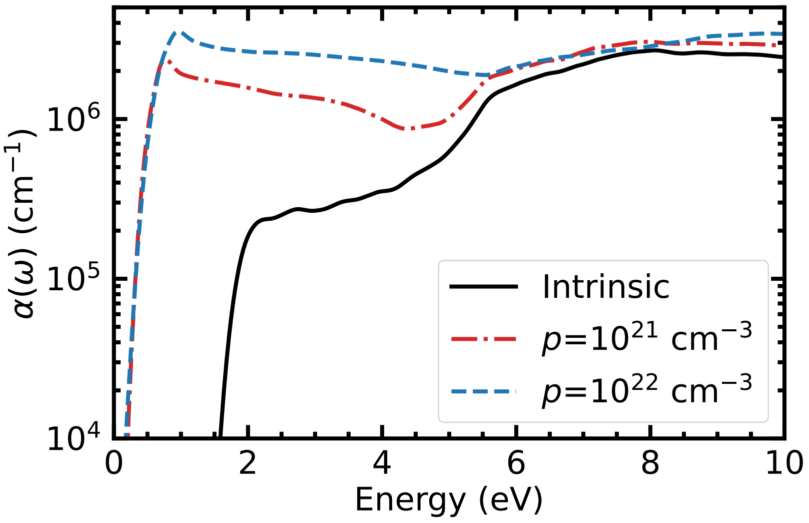


FIG. S3. Calculated absorption coefficient of $c$-BeB$_2$ under different doping conditions. Notably, strong absorption is always seen above a photon energy of 2 eV.

## IV. PHONON DISPERSION OF $c$-BEB$_2$ WITH JELLIUM MODEL

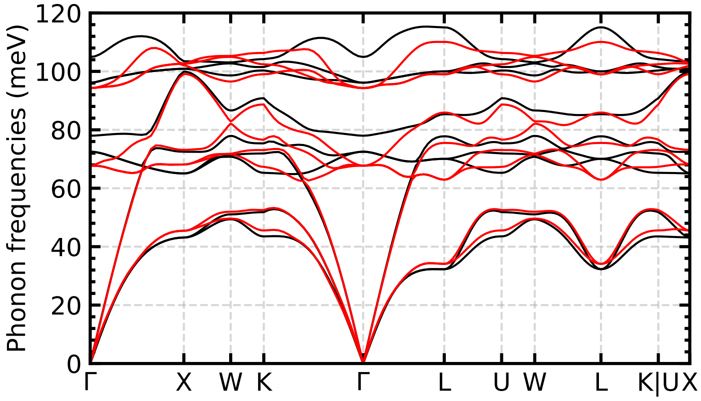


FIG. S4. Phonon dispersion relationship of $c$-BeB$_2$ for the undoped system (black) versus that from the jellium model corresponding to a doping level of $9.8 \times 10^{21}$ cm$^{-3}$ (red). Within the jellium model, mainly the optical phonon frequencies are affected and the LO-TO splitting vanishes due to the metallic screening.
